# Supplementary material for: Where is my Wallet? Modeling Object Proposal Sets for Egocentric Visual Query Localization
Source: arXiv:2211.10528 source file (2023-04-06)
Supplement: Supplementary file 1 [file Supplementary.tex]

% CVPR 2023 Paper Template
% based on the CVPR template provided by Ming-Ming Cheng (https://github.com/MCG-NKU/CVPR_Template)
% modified and extended by Stefan Roth (stefan.roth@NOSPAMtu-darmstadt.de)

\documentclass[10pt,twocolumn,letterpaper]{article}

%%%%%%%%% PAPER TYPE  - PLEASE UPDATE FOR FINAL VERSION
\usepackage[review]{cvpr}      % To produce the REVIEW version
%\usepackage{cvpr}              % To produce the CAMERA-READY version
%\usepackage[pagenumbers]{cvpr} % To force page numbers, e.g. for an arXiv version

% Include other packages here, before hyperref.
\usepackage{graphicx}
\usepackage{amsmath}
\usepackage{amssymb}
\usepackage{booktabs}
\usepackage{multirow}
\usepackage{adjustbox}
\usepackage{sidecap}
\usepackage{float}

\usepackage{pifont}%
% It is strongly recommended to use hyperref, especially for the review version.
% hyperref with option pagebackref eases the reviewers' job.
% Please disable hyperref *only* if you encounter grave issues, e.g. with the
% file validation for the camera-ready version.
%
% If you comment hyperref and then uncomment it, you should delete
% ReviewTempalte.aux before re-running LaTeX.
% (Or just hit 'q' on the first LaTeX run, let it finish, and you
%  should be clear).
\usepackage[pagebackref,breaklinks,colorlinks]{hyperref}

\usepackage[dvipsnames]{xcolor}
% Support for easy cross-referencing
\usepackage[capitalize]{cleveref}
\crefname{section}{Sec.}{Secs.}
\Crefname{section}{Section}{Sections}
\Crefname{table}{Table}{Tables}
\crefname{table}{Tab.}{Tabs.}

%%%%%%%%% PAPER ID  - PLEASE UPDATE
 % *** Enter the CVPR Paper ID here

% \newcommand{\JM}[1]{{{#1}}}
% \newcommand{\FX}[1]{{#1}}
%
%

\begin{document}

%%%%%%%%% TITLE - PLEASE UPDATE
%\title{Modeling Egocentric Object in the Wild for Visual Query Localization}
\title{Where is my Wallet? Modeling Object Proposal Sets\\ for Egocentric Visual Query Localization \\  --- \textit{supplementary material} --- }

\author{First Author\\
Institution1\\
Institution1 address\\
{\tt\small firstauthor@i1.org}
% For a paper whose authors are all at the same institution,
% omit the following lines up until the closing ``}''.
% Additional authors and addresses can be added with ``\and'',
% just like the second author.
% To save space, use either the email address or home page, not both
\and
Second Author\\
Institution2\\
First line of institution2 address\\
{\tt\small secondauthor@i2.org}
}
\maketitle

% \begin{abstract}
% \input{section/00_abstract.tex}
% \end{abstract}

%%%%%%%%% SECTIONS
\renewcommand\thesection{\Alph{section}}
\input{section/09_appendix.tex}

%%%%%%%%% REFERENCES
{\small
\bibliographystyle{ieee_fullname}
\bibliography{egbib}
}

\end{document}
